# Supplementary material for: Human101: Training 100+FPS Human Gaussians in 100s from 1 View
Source: arXiv:2312.15258 source file (2023-12-23)
Supplement: Supplementary file 1 [file _supplementary.tex]

\input{_constants}
\review % \review OR \cameraready

\documentclass[10pt,twocolumn,letterpaper]{article}
\input{cvpr_header}
\myexternaldocument{_main}
\begin{document}

%% TITLE
\title{\paperTitle}
\author{\authorBlock}
\maketitlesupplementary

\input{12_appendix}

{\small
\bibliographystyle{ieee_fullname}
\bibliography{11_references}
}

\end{document}
